# Supplementary material for: Variational Diffusion Posterior Sampling with Midpoint Guidance
Source: arXiv:2410.09945 source file (2024-12-24)
Supplement: Supplementary file 1 [file _gaussian_case.tex]

\section{Gaussian Case}

\subsection*{DDM for Gaussian}
Here, the prior is Gaussian $\prior(\bx _0) = \normpdf (\bx _0; \mu, \sigma^2 \Id)$.
In this case, DDM can be explicitly derived, namely the
\begin{equation}
    \begin{aligned}
        \text{marginals} & \quad
            \fwmarg{k}{}(\bx _k) = \normpdf \big( \bx _k; \sqrt{\acp{k}} \mu, (\var_k + \acp{k} \sigma^2) \Id \big), \\
        \text{denoising densities} & \quad
            \bw{0|k}{\bx _k}{\bx _0} = \normpdf(\bx _0;
                % mean
                \underbrace{\frac{\sqrt{\acp{k}}\sigma^2}{\var_k + \acp{k}\sigma^2} \bx _k + \frac{\var_k}{\var_k + \acp{k}\sigma^2} \mu}_{\mu_{0|k}(\bx _k)},
                % var
                \underbrace{\frac{\var_k \sigma^2}{\var_k + \acp{k}\sigma^2}}_{\sigma_{0|k}^2} \Id)
    \end{aligned}
    \enspace.
\end{equation}
Notice the mean $\mu_{0|k}(\bx _k)$ is linear in $\bx _k$.
Building upon the latter formulas, we derive the expressions of the score and the denoiser
\begin{align}
    s_t(\bx _k) = -\frac{\bx _k - \sqrt{\acp{k}} \mu}{\var_k + \acp{k}\sigma^2}, \quad
    \pE[\bX _0 | \bx _k] = \mu_{0|k}(\bx _k)
    \enspace.
\end{align}

\subsection*{likelihood for linear inverse problems}
The likelihood $\potn{}{}$ defined by a linear inverse problem
\begin{equation}
    y = A \bx _0 + \sigma_y \beps, \quad
    A \in \rset^{d \times d}, \sigma_y > 0, \mathrm{and} \ \beps \sim \normpdf(0, \Id)
    \enspace,
\end{equation}
reads $\potn{}{\bx _0} = \normpdf(y; A \bx _0, \sigma^2 \Id)$.
Under the assumption of Gaussian prior, we can establish the expression of the intermediate likelihoods $\potn{k}{\bx _k}$
\begin{equation}
    \begin{aligned}
        \potn{k}{\bx _k}
            & = \int \potn{}{\bx _0} \bw{0|k}{\bx _k}{\bx _0} \rmd \bx _0 \\
            & = \normpdf(y; A \mu_{0|k}(\bx _k), \sigma_y^2 \Id + \sigma_{0|k}^2 A A^\top)
    \end{aligned}
    \enspace,
\end{equation}
In parallel, the approximate intermediate likelihoods are
\begin{equation}
    \hpotn{k}{\bx _k} = \potn{}{\pE[\bX _0 | \bx _k]} = \normpdf(y; A \mu_{0|k}(\bx _k), \sigma_y^2 \Id)
    \enspace.
\end{equation}
Notice that $\potn{k}{}$ and $\hpotn{k}{}$ differ only in the variance with $\potn{k}{}$ having an extra term in the variance.

\subsection*{Variational approximation}

Learning the mean of the Gaussian variational approximation
\begin{equation}
    \vpibw{\tmid{k}|k+1}{\bx _{k+1}}{\bx _{\tmid{k}}} = \normpdf(\bx _{\tmid{k}}; \varphi, \sigma^2_{\tmid{k}|k+1, 0} \Id)
    \enspace,
\end{equation}
of $\hpibw{\tmid{k}|k+1}{\bx _{k+1}}{\cdot}[]$ reduces to minimizing the following objective function
\begin{equation}
        - \pE[\log \hpotn{\tmid{k}}{\bx _\tmid{k}} ]
        - \pE[\fwtrans{k+1|\tmid{k}}{\bx _{\tmid{k}}}{\bx _{k+1}}]
        - \pE[\log  \fwmarg{\tmid{k}}{}(\bx _{\tmid{k}}) ]
        \enspace,
\end{equation}
where the expected value is taken \wrt \ $\vpibw{\tmid{k}|k+1}{\bx _{k+1}}{\cdot}$.
Since we are not optimizing over the variance, this objective equals up to a constant \wrt \ $\varphi$ to the following
\begin{equation}
    \mathcal{L}_\tmid{k}(\varphi; \bx _{k+1}) =
    \frac{\| y - A \mu_{0|\tmid{k}}(\varphi) \|^2}{2 \sigma_y^2}
    + \frac{ \| \bx _{k+1} -  \sqrt{\frac{\acp{k+1}}{\acp{\tmid{k}}}} \varphi \|^2 }{2 (1 - \frac{\acp{k+1}}{\acp{\tmid{k}}})}
    + \frac{ \| \varphi - \sqrt{\acp{\tmid{k}}} \mu \|^2 }{2 (\var_{\tmid{k}} + \acp{\tmid{k}}\sigma^2)}
    \enspace.
\end{equation}
This objective function is quadratic hence the optimal variational parameter that minimizes it is
\begin{equation}
    \hat{\varphi}(\bx _{k+1}) = -[\nabla_{\varphi}^2 \mathcal{L}_\tmid{k}]^{-1} \nabla_{\varphi} \mathcal{L}_\tmid{k}(0; \bx _{k+1})
    \enspace.
\end{equation}
where $\nabla_{\varphi}^2 \mathcal{L}_\tmid{k}$ is the Hessian and is constant and independent of $\bx _{k+1}$. On the other hand, the gradient depends linearly on $\bx _{k+1}$ and the term in front of it is $\nabla_{\bx _{k+1}} [\nabla_{\varphi} \mathcal{L}_\tmid{k}(0; \bx _{k+1})] =- \frac{ \sqrt{\acp{k+1} / \acp{\tmid{k}}}}{2 (1 - \acp{k+1} / \acp{\tmid{k}})} \Id$.

\subsection*{Mean and covariance of the approximate marginals}

The variational backward is a Gaussian as it is a convolution of two Gaussian distributions
\begin{equation}
    \vpibw{k|k+1}{\bx _{k+1}}{\bx _k} = \int \fwtrans{k|\tmid{k}, k+1}{\bx _\tmid{k}, \bx _{k+1}}{\bx _k} \vpibw{\tmid{k}|k+1}{\bx _{k+1}}{\bx _\tmid{k}} \, \rmd \bx _{\tmid{k}}
    \enspace,
\end{equation}
Knowing that $\fwtrans{k|\tmid{k}, k+1}{\bx _\tmid{k}, \bx _{k+1}}{\bx _k} = \normpdf(\bx _k; a_{k|\tmid{k},k+1} \bx _{k+1} + b_{k|\tmid{k},k+1} \bx _{\tmid{k}}, \sigma^2_{k|\tmid{k},k+1} \Id)$, we have
\begin{equation}
    \begin{aligned}
        \pE[\bX _k | \bx _{k+1}]
            & = a_{k|\tmid{k},k+1} \bx _{k+1} + b_{k|\tmid{k},k+1} \hat{\varphi}(\bx _{k+1}) \\
        \pV[\bX _k | \bx _{k+1}]
            & =  \big( (b_{k|\tmid{k},k+1} \sigma_{\tmid{k}|k+1,0})^2 + \sigma^2_{k|\tmid{k},k+1} \big) \Id
    \end{aligned}
    \enspace,
\end{equation}
where the expected value $\pE$ and variance $\pV$ are taken \wrt \  $\vpibw{k|k+1}{\bx _{k+1}}{\cdot}$.
Marginalizing over $\bX _{k+1} \sim \vpibw{k+1}{}{}$, we obtain the following recursion
\begin{equation}
    \begin{aligned}
        \pE[\bX _k]
            & = a_{k|\tmid{k},k+1} \pE[\bX _{k+1}] + b_{k|\tmid{k},k+1} \hat{\varphi} \big( \pE[\bX _{k+1}] \big), \\
        \pV[\bX _k]
            & = M_{\tmid{k}} \pV[\bX _{k+1}] M_{\tmid{k}}^\top +  \big( (b_{k|\tmid{k},k+1} \sigma_{\tmid{k}|k+1,0})^2 + \sigma^2_{k|\tmid{k},k+1} \big) \Id, \\
        \pE[\bX _n] & = 0,  \pV[\bX _n] = \Id,
    \end{aligned}
\end{equation}
where $M_{\tmid{k}} = a_{k|\tmid{k},k+1} \Id + \frac{ \sqrt{\acp{k+1} / \acp{\tmid{k}}}}{2 (1 - \acp{k+1} / \acp{\tmid{k}})}  b_{k|\tmid{k},k+1} \nabla_{\varphi}^2 \mathcal{L}_\tmid{k}$.
