# Supplementary material for: Variational Diffusion Posterior Sampling with Midpoint Guidance
Source: arXiv:2410.09945 source file (2024-12-24)
Supplement: Supplementary file 2 [file _stale_proofs.tex]

\section{Proofs}
\label{apdx:proofs}
\subsection{Proof of XXX}
In this section we assume that $\potn{}{\bx} = \normpdf(\obs; Ax, \stdobs^2 \Id)$. We proceed to bound
$$
    \kldivergence{\pibw{\ell|k}{\bx _k}{\cdot}}{\hpibw{\ell|k}{\bx _k}{\cdot}[]} \eqsp.
$$
We have that
\begin{multline*}
    \kldivergence{\pibw{\ell|k}{\bx _k}{\cdot}}{\hpibw{\ell|k}{\bx _k}{\cdot}[]} \\
    = \int \log \frac{\potn{\ell}{\bx _\ell}}{\hpotn{\ell}{\bx _\ell}} \pibw{\ell|k}{\bx _k}{\bx _\ell} \, \rmd \bx _\ell - \log \potn{k}{\bx _k} + \log \int \hpotn{\ell}{\bx _\ell} \bw{\ell|k}{\bx _k}{\bx _\ell} \, \rmd \bx _\ell \eqsp.
\end{multline*}
For the first term, by convexity of $\bx \mapsto \bx \log \bx$ and then definition of $\potn{\ell}{}$, it follows by Jensen's inequality that
\begin{align*}
    \int \log \frac{\potn{\ell}{\bx _\ell}}{\hpotn{\ell}{\bx _\ell}} \pibw{\ell|k}{\bx _k}{\bx _\ell} \, \rmd \bx _\ell & = \int \log \frac{\potn{\ell}{\bx _\ell}}{\hpotn{\ell}{\bx _\ell}} \frac{\potn{\ell}{\bx _\ell} \bw{\ell|k}{\bx _k}{\bx _\ell}}{\potn{k}{\bx _k}} \, \rmd \bx _\ell \\
    & \leq \int \log \frac{\potn{}{\bx _0}}{\hpotn{\ell}{\bx _\ell}} \pibw{0, \ell|k}{\bx _k}{\bx _0, \bx _\ell} \, \rmd \bx _0 \rmd \bx _\ell \eqsp.
\end{align*}
where $\pibw{0, \ell|k}{\bx _k}{\bx _0, \bx _\ell} = \potn{}{\bx _0} \bw{0|\ell}{\bx _\ell}{\bx _0} \bw{\ell|k}{\bx _k}{\bx _\ell} \big/ \potn{k}{\bx _k}$ and is a probability measure.
Next, it holds that
\begin{align}
    \int \log \potn{}{\bx _0} \pibw{0, \ell|k}{\bx _k}{\bx _0} \, \rmd \bx _0 & = - \frac{1}{2 \stdobs^2 }\int \| \obs - A \bx _0 \|^2 \pibw{0|\ell}{\bx _\ell}{\bx _0} \, \rmd \bx _0 \\
    & =
\end{align}
\subsection{Useful computations}
In what follows we assume that $\prior(\bx) = \normpdf(\bx; \zero_\dimx, \Id_\dimx)$ and $\potn{}{\bx} = \normpdf(\obs, A \bx, \stdobs^2 \Id_\dimobs)$. $A \in \rset^{\dimobs \times \dimx}$ is a diagonal rectangular matrix with diagonal $(s_1, \dotsc, s_\dimobs)$. Following \cite[Eq. 2.116]{bishop2006pattern} we have that
$$
    \pi(\bx) = \normpdf(\bx; \Sigma_\obs A^\intercal \obs / \stdobs^2, \Sigma_\obs)
$$
where $\Sigma_\obs = \mathrm{diag}(\var{\obs, 1}, \dotsc, \var{\obs, \dimx})$ where $\var{\obs, i} = \stdobs^2 / (\stdobs^2 + s^2 _i)$ for $\intset{1}{\dimobs}$ and $\var{\obs, i} = 1$ otherwise.

Define $\acp{k| \ell} \eqdef \acp{k} / \acp{\ell}$, $\var{k|\ell} \eqdef 1 - \acp{k|\ell}$. Following the definitions in the main paper we have for all $\ell \in \intset{0}{k-1}$,
$$
   \bw{\ell|k}{\bx _k}{\bx _\ell} = \normpdf(\bx _\ell; \sqrt{\acp{k|\ell}} \bx _k, 1 - \acp{k|\ell}) \eqsp.
$$
Next, the true likelihood $\potn{k}{}$ and approximate DPS likelihood $\hpotn{k}{}$ are defined for all $k \in \intset{0}{n}$ by
\begin{align}
    \potn{k}{\bx _k} & = \normpdf(\obs; \sqrt{\acp{k}} A \bx _k , \Sigma^y _k) \eqsp,\\
    \hpotn{k}{\bx _k} &= \normpdf(\obs; \sqrt{\acp{k}} A \bx _k , \stdobs^2 \Id_\dimobs)
\end{align}
where $\Sigma^y _k = \var{0|k} AA^\intercal + \stdobs^2 \Id_\dimobs$.
Hence, the only difference between the true likelihood and the approximate one lies in the covariance matrix.

Next, for all $\ell, k$ such that $\ell < k$,
\begin{align}
    \hpibw{\ell|k}{\bx _k}{\bx _\ell}[] = \normpdf\big(\bx _\ell;  \mean{\ell|k}^\obs(\bx _k) , \hat\Sigma^\obs _{\ell|k}\big)
\end{align}
where
$$
    \mean{\ell|k}^\obs(\bx _k) \eqdef \hat\Sigma^\obs _{\ell|k} \big\{(\sqrt{\acp{\ell}} / \stdobs^2) A^\intercal \obs+ (\sqrt{\acp{k|\ell}} / \var{k|\ell}) \bx _k\big\}
$$
and $\hat\Sigma^\obs _{\ell|k}$ is a diagonal matrix and $(\hat\Sigma^\obs _{\ell|k})_{i,i} = \frac{\var{k|\ell} \stdobs^2}{\stdobs^2 + s^2 _i \var{k|\ell} \acp{\ell}}$ if $i \leq \dimobs$ and $(\hat\Sigma^\obs _{\ell|k})_{i, i} = \var{k|\ell}$ otherwise. As a result,
$$
    \hpibw{k|k+1}{\bx _{k+1}}{\bx _k}[] = \normpdf\big(\bx _k; \big)
$$
