# Supplementary material for: Variational Diffusion Posterior Sampling with Midpoint Guidance
Source: arXiv:2410.09945 source file (2024-12-24)
Supplement: Supplementary file 3 [file DPS_pitfall.tex]

\section{Numerical study of DPS-like likelihood approximations}
\label{sec:study_appro\bx _DPS}

We preface this section by an informal discussion on the fact that DPS-like likelihood approximations deteriorates with $k$.
